# Supplementary material for: Effects of Critical Point on Quark Gluon Plasma
Source: arXiv:2307.14601 source file (2023-07-27)
Supplement: Supplementary file 1 [file CH04_appendix1.tex]

\chapter[Entropy density of QGP and hadrons]{Equation of state with critical point}
\label{appendix04_A}
\subsection{Another way to calculate entropy density:}
The free energy can be written as the grand canonical partition function$(\mathcal{Z})$ of the non-interacting relativistic gas if particles and anti-particles is given by 
\beqa
\Omega &=& -Tln\mathcal{Z}= \frac{TVg\epsilon}{2\pi^2}\int\limits_{0}^{\infty} dp p^2 [ln(1+\epsilon e^{-\beta(\sqrt{p^2+m^2}-\mu)})+ln(1+\epsilon e^{-\beta(\sqrt{p^2+m^2}+\mu)})]
\eeqa
Now
\beq
ln(1+x)=\sum_{n=1}^{\infty}\frac{(-1)^{n+1}}{n} x^n
\eeq
Thus
\beqa
\Omega  &=& -\frac{TVg\epsilon}{2\pi^2}\int\limits_{0}^{\infty} dp p^2 \sum_{n=1}^{\infty}\frac{(-1)^{n+1}}{n}[\{\epsilon e^{-\beta(\sqrt{p^2+m^2}-\mu)}\}^n+\{\epsilon e^{-\beta(\sqrt{p^2+m^2}+\mu)}\}^n] \nonumber\\
% % % % % % %
&=& -\frac{TVg\epsilon}{2\pi^2}\int\limits_{0}^{\infty} dp p^2 \sum_{n=1}^{\infty}\frac{(-1)^{n+1}}{n}[\{\epsilon^n e^{-n\beta(\sqrt{p^2+m^2}-\mu)}\}+\{\epsilon^n e^{-n\beta(\sqrt{p^2+m^2}+\mu)}\}] \nonumber\\ 
% % % % %% % %
&=&- \frac{TVg\epsilon}{2\pi^2} \sum_{n=1}^{\infty}\frac{(-1)^{n+1}}{n}\epsilon^n \int\limits_{0}^{\infty} dp p^2[e^{-n\beta(E_i-\mu)}+ e^{-n\beta(E_i+\mu)}] \nonumber\\
% % % % % % % %
&=& -\frac{TVg\epsilon}{2\pi^2} \sum_{n=1}^{\infty}\frac{(-1)^{n+1}}{n}\epsilon^n \int\limits_{0}^{\infty} dp p^2[e^{-n\beta E_i} e^{n\beta \mu}+ e^{-n\beta E_i} e^{-n\beta \mu}]
\eeqa
\beqa
d^3p &=& 4\pi p^2 dp \nonumber\\
p^2dp&=& \frac{d^3p}{4\pi}
\eeqa
\beqa
\Omega  &=& \frac{TVg\epsilon}{8\pi^3} \sum_{n=1}^{\infty}\frac{(-1)^{n+1}}{n}\epsilon^n [e^{n\beta \mu} \int\limits_{0}^{\infty} d^3p e^{-n\beta E_i}+e^{-n\beta \mu} \int\limits_{0}^{\infty} d^3p e^{n\beta E_i}]
\eeqa
\textbf{Bessel's functions:}\\
\beqa
K_n(z) &=& \frac{2^n n!}{(2n)! z^n}\int d\tau e^{-\tau} (\tau^2-z^2)^{n-\frac{1}{2}} \nonumber\\
K_n(z) &=& \frac{2^{n-1} (n-1)!}{(2n-2)! z^n}\int d\tau (\tau e^{-\tau}) (\tau^2-z^2)^{n-\frac{3}{2}}
\eeqa
Thus
\beq
K_2(z)=\frac{1}{z^2}\int d\tau (\tau e^{-\tau}) (\tau^2-z^2)^{\frac{1}{2}}
\eeq
Back to main calculation, we put
\beqa
z_i=\frac{m_i}{T}\rightarrow m_i=Tz_i;\hspace*{0.7cm} \tau_i=\frac{E_i}{T}=\frac{\sqrt{p^2_i+m^2_i}}{T}\rightarrow \hspace*{0.2cm} E_i=T\tau_i
\eeqa
\beqa
p_i=T\sqrt{\tau^2-z^2}\rightarrow p^2_i=T^2(\tau^2-z^2) \rightarrow p_i dp_i=T^2\tau_i d\tau_i
\eeqa
\beqa
d^3p=4\pi p^2dp=4\pi p p dp &=& 4\pi\sqrt{T^2(\tau^2-z^2)} T^2\tau_i d\tau_i \nonumber\\
&=& 4\pi T^3\sqrt{\tau^2-z^2}\tau_i d\tau_i
\eeqa
So
\beqa
\int\limits_{0}^{\infty}d^3p e^{-n\beta E_i} &=& 4\pi \int\limits_{0}^{\infty} p^2_i dp_i e^{-n\beta E_i} \nonumber\\
&=& 4\pi T^3 \int\limits_{0}^{\infty} d\tau_i  \tau_i \sqrt{\tau^2-z^2} e^{-n\beta E_i} \nonumber\\
&=& 4\pi T^3 \int\limits_{0}^{\infty} d\tau_i  \tau_i \sqrt{\tau^2-z^2} e^{-\frac{n}{T}T\tau_i} \nonumber\\
&=& 4\pi T^3 \int\limits_{0}^{\infty} d\tau_i  \tau_i \sqrt{\tau^2-z^2} e^{-n\tau_i} \nonumber\\
&=& 4\pi T^3\frac{1}{n^3} \int\limits_{0}^{\infty}(n\tau_i)\sqrt{(n\tau_i)^2-(nz)^2} e^{-n\tau_i} d(n\tau_i) \nonumber\\
&=& \frac{4\pi T^3}{n^3}(nz)^2\times \frac{1}{(nz)^2}\int\limits_{0}^{\infty} (n\tau_i)\{(n\tau_i)^2-(nz)^2\}^{\frac{1}{2}} e^{-n\tau_i} d(n\tau_i)  \nonumber\\
&=& \frac{4\pi T^3}{n^3}(nz)^2 K_2(nz)
\eeqa
Finally, the free energy can be written as
\beqa
\Omega &=& -Tln\mathcal{Z} \nonumber\\
&=& - \frac{TVg\epsilon}{8\pi^3} \sum_{n=1}^{\infty}\frac{(-1)^{n+1}}{n}\epsilon^n [e^{n\beta \mu} \int\limits_{0}^{\infty} d^3p e^{-n\beta E_i}+e^{-n\beta \mu} \int\limits_{0}^{\infty} d^3p e^{n\beta E_i}] \nonumber\\
&=& -\frac{TVg\epsilon}{8\pi^3} \sum_{n=1}^{\infty}\frac{(-1)^{n+1}}{n}\epsilon^n  \{e^{n\beta \mu}+e^{-n\beta \mu}\} \int\limits_{0}^{\infty} d^3p e^{-n\beta E_i} \nonumber\\
&=& -\frac{TVg\epsilon}{8\pi^3} \sum_{n=1}^{\infty}\frac{(-1)^{n+1}}{n}\epsilon^n cosh(n\beta \mu) \frac{4\pi T^3}{n^3}(nz)^2 K_2(nz) \nonumber\\
&=& -\frac{gVT^4}{2\pi^2} \sum_{n=1}^{\infty}\frac{(-1)^{n+1}}{n^4} cosh(n\beta \mu) (\frac{nm_i}{T})^2 K_2(\frac{nm_i}{T})
\eeqa
where we have put $\epsilon$ to be 1.\\
Now the free energy $\Omega$ is defined as 
\beqa
\Omega &=& E-TS \nonumber\\
d\Omega &=& dE-TdS-SdT \nonumber\\
\eeqa
Thus
\beqa
S &=& -(\frac{\partial \Omega}{\partial T}) \nonumber\\
&=& -\frac{\partial }{\partial T}(-KTln \mathcal{Z}) 
\eeqa
\beq
\begin{aligned}
S = \frac{2gVT^3}{\pi^2} \sum_{n=1}^{\infty}\frac{(-1)^{n+1}}{n^4} cosh(n\beta \mu) (\frac{nm_i}{T})^2 K_2(\frac{nm_i}{T}) 
% % % % % % % % % % % % %
\\-\frac{gV\mu T^2}{2\pi^2K} \sum_{n=1}^{\infty}\frac{(-1)^{n+1}}{n^3} sinh(n\beta \mu) (\frac{nm_i}{T})^2 K_2(\frac{nm_i}{T})
% % % % % % % % % % % % %
\\-\frac{gVT}{\pi^2} \sum_{n=1}^{\infty}\frac{(-1)^{n+1}}{n^2} cosh(n\beta \mu) m^2_i K_2(\frac{nm_i}{T})
% % % % % % % % % % % % %
\\-\frac{gVT^4}{4\pi^2} \sum_{n=1}^{\infty}\frac{(-1)^{n+1}}{n^4} cosh(n\beta \mu) (\frac{nm_i}{T})^2 [K_1(\frac{nm_i}{T}) +K_3(\frac{nm_i}{T})]
\end{aligned}
\eeq
This is the entropy density for hadrons.
